# Supplementary material for: Deformable NeRF using Recursively Subdivided Tetrahedra
Source: arXiv:2410.04402 source file (2024-10-06)
Supplement: Supplementary file 1 [file DeformRF_MM2024_CameraReady_supp.pdf]

# Supplementary Materials: DeformRF

## 1 Hierarchical Barycentric Inference

This section delves into the hierarchical barycentric inference within a tetrahedral mesh, emphasizing two pivotal processes given the barycentric coordinates  $\alpha^\ell = (\alpha_0^\ell, \alpha_1^\ell, \alpha_2^\ell, \alpha_3^\ell)$  of a sampling point  $\mathbf{p}$  at level  $\ell$ : the determination of the specific child tetrahedron containing  $\mathbf{p}$ , and the computation of the barycentric coordinates at the subsequent level  $\ell + 1$ .

Note that we select a specific subdivision pattern and uniformly apply this pattern to all tetrahedra in the mesh, as shown in Fig. 1.

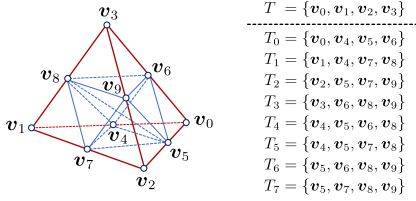

**Figure 1: Subdivision of a Tetrahedron.** Given a tetrahedron  $T$ , we subdivide it into eight smaller tetrahedra  $T_k$ , for  $k \in \{0, \dots, 7\}$ , by connecting the midpoints of each edge.

Now we consider an arbitrary tetrahedron in level  $\ell$  defined by its four vertices  $\mathbf{v}_0^\ell, \mathbf{v}_1^\ell, \mathbf{v}_2^\ell, \mathbf{v}_3^\ell \in \mathbb{R}^3$ . For a given sampling point  $\mathbf{p}$  located within this tetrahedron, assume its barycentric coordinate in level  $\ell$  is known and denoted as  $\alpha^\ell = (\alpha_0^\ell, \alpha_1^\ell, \alpha_2^\ell, \alpha_3^\ell)$ . The coordinates of  $\mathbf{p}$  can thus be expressed as:

$$\mathbf{p} = \alpha_0^\ell \mathbf{v}_0^\ell + \alpha_1^\ell \mathbf{v}_1^\ell + \alpha_2^\ell \mathbf{v}_2^\ell + \alpha_3^\ell \mathbf{v}_3^\ell. \quad (1)$$

First of all, we need to determine the specific child tetrahedron containing the sampling point  $\mathbf{p}$ . Upon subdividing the original tetrahedron by connecting these midpoints as shown in Fig. 1, we apply a set of criteria as follows:

- (1)  $\alpha_0^\ell \geq 0.5$ ,      (2)  $\alpha_1^\ell \geq 0.5$ ,
- (3)  $\alpha_2^\ell \geq 0.5$ ,      (4)  $\alpha_3^\ell \geq 0.5$ ,
- (5)  $\begin{cases} \alpha_i^\ell < 0.5 \text{ for } i \in \{0, 1, 2, 3\}, \\ \alpha_1 + \alpha_2 < 0.5, \\ \alpha_2 + \alpha_3 < 0.5, \end{cases}$
- (6)  $\begin{cases} \alpha_i^\ell < 0.5 \text{ for } i \in \{0, 1, 2, 3\}, \\ \alpha_1 + \alpha_2 \geq 0.5, \\ \alpha_2 + \alpha_3 < 0.5, \end{cases}$
- (7)  $\begin{cases} \alpha_i^\ell < 0.5 \text{ for } i \in \{0, 1, 2, 3\}, \\ \alpha_1 + \alpha_2 < 0.5, \\ \alpha_2 + \alpha_3 \geq 0.5, \end{cases}$
- (8)  $\begin{cases} \alpha_i^\ell < 0.5 \text{ for } i \in \{0, 1, 2, 3\}, \\ \alpha_1 + \alpha_2 \geq 0.5, \\ \alpha_2 + \alpha_3 \geq 0.5. \end{cases}$

Based on the criteria outlined above, we devised the following algorithm to effectively implement these conditions. We show the pseudo code in Algorithm 1. This algorithm is specifically designed to determine the placement of a sampling point within a subdivided tetrahedron. By evaluating the barycentric coordinates relative to the established thresholds, the algorithm identifies which of the eight possible child tetrahedra contains the point.

---

### Algorithm 1 Determine Child Tetrahedron for Sampling Point

---

**Input:** Barycentric coordinates  $\alpha^\ell = (\alpha_0^\ell, \alpha_1^\ell, \alpha_2^\ell, \alpha_3^\ell)$  of point  $\mathbf{p}$  in tetrahedron defined by vertices  $\mathbf{v}_0^\ell, \mathbf{v}_1^\ell, \mathbf{v}_2^\ell, \mathbf{v}_3^\ell$ .

**Output:** Index of child tetrahedron containing  $\mathbf{p}$ .

1: Initialize index of child tetrahedron  $i_c \leftarrow -1$

2: **if**  $\alpha_0^\ell \geq 0.5$  **then**

3:      $i_c \leftarrow 0$

4: **else if**  $\alpha_1^\ell \geq 0.5$  **then**

5:      $i_c \leftarrow 1$

6: **else if**  $\alpha_2^\ell \geq 0.5$  **then**

7:      $i_c \leftarrow 2$

8: **else if**  $\alpha_3^\ell \geq 0.5$  **then**

9:      $i_c \leftarrow 3$

10: **else**

11:     Compute conditions based on sums:

12:      $\text{flag1} \leftarrow (\alpha_1^\ell + \alpha_2^\ell < 0.5)$

13:      $\text{flag2} \leftarrow (\alpha_2^\ell + \alpha_3^\ell < 0.5)$

14:     **if**  $\text{flag1} \wedge \text{flag2}$  **then**

15:          $i_c \leftarrow 4$

16:     **else if**  $\neg \text{flag1} \wedge \text{flag2}$  **then**

17:          $i_c \leftarrow 5$

18:     **else if**  $\text{flag1} \wedge \neg \text{flag2}$  **then**

19:          $i_c \leftarrow 6$

20:     **else**

21:          $i_c \leftarrow 7$

22:     **end if**

23: **end if**

24: **return**  $i_c$

---

Let the barycentric coordinates of  $\mathbf{p}$  in the specific child tetrahedron be  $\alpha^{\ell+1} = (\alpha_0^{\ell+1}, \alpha_1^{\ell+1}, \alpha_2^{\ell+1}, \alpha_3^{\ell+1})$ . For each of the eight child configurations resulting from the subdivision of a parent tetrahedron, a coefficient matrix  $\mathbf{C}_i \in \mathbb{R}^{4 \times 4}$ , where  $i = 0, \dots, 7$ , can be defined such that  $\alpha^{\ell+1} = \mathbf{C}_i \alpha^\ell$ .

We now proceed to derive the coefficient matrices  $\mathbf{C}_i$ , focusing on  $\mathbf{C}_4$  as an illustrative example. Assuming that the sampling point  $\mathbf{p}$  is located within the child tetrahedron  $T_4$ , the position of  $\mathbf{p}$  can be represented as a linear combination of the vertices defining  $T_4$ :

$$\mathbf{p} = \alpha_0^{\ell+1} \mathbf{v}_4 + \alpha_1^{\ell+1} \mathbf{v}_5 + \alpha_2^{\ell+1} \mathbf{v}_6 + \alpha_3^{\ell+1} \mathbf{v}_8. \quad (2)$$

Since the vertices  $\mathbf{v}_4, \mathbf{v}_5, \mathbf{v}_6$ , and  $\mathbf{v}_8$  are midpoints in tetrahedron  $T_4$ , we express them as  $\frac{1}{2} \mathbf{v}_0 + \frac{1}{2} \mathbf{v}_1$ ,  $\frac{1}{2} \mathbf{v}_0 + \frac{1}{2} \mathbf{v}_2$ ,  $\frac{1}{2} \mathbf{v}_0 + \frac{1}{2} \mathbf{v}_3$  and  $\frac{1}{2} \mathbf{v}_1 + \frac{1}{2} \mathbf{v}_3$ , respectively. We then obtain the following equation:

$$\begin{aligned}
\mathbf{p} &= \alpha_0^{\ell+1} \left( \frac{1}{2} \mathbf{v}_0 + \frac{1}{2} \mathbf{v}_1 \right) + \alpha_1^{\ell+1} \left( \frac{1}{2} \mathbf{v}_0 + \frac{1}{2} \mathbf{v}_2 \right) + \alpha_2^{\ell+1} \left( \frac{1}{2} \mathbf{v}_0 + \frac{1}{2} \mathbf{v}_3 \right) \\
&\quad + \alpha_3^{\ell+1} \left( \frac{1}{2} \mathbf{v}_1 + \frac{1}{2} \mathbf{v}_3 \right) \\
&= \frac{1}{2} \left( \alpha_0^{\ell+1} + \alpha_1^{\ell+1} + \alpha_2^{\ell+1} \right) \mathbf{v}_0 + \frac{1}{2} \left( \alpha_0^{\ell+1} + \alpha_3^{\ell+1} \right) \mathbf{v}_1 + \frac{1}{2} \alpha_1^{\ell+1} \mathbf{v}_2 \\
&\quad + \frac{1}{2} \left( \alpha_2^{\ell+1} + \alpha_3^{\ell+1} \right) \mathbf{v}_3.
\end{aligned}$$

Recall Eq. (1), therefore the equations relating  $\alpha^\ell$  and  $\alpha^{\ell+1}$  are:

$$\begin{cases} \frac{1}{2}(\alpha_0^{\ell+1} + \alpha_1^{\ell+1} + \alpha_2^{\ell+1}) = \alpha_0 \\ \frac{1}{2}(\alpha_0^{\ell+1} + \alpha_3^{\ell+1}) = \alpha_1 \\ \frac{1}{2}\alpha_1^{\ell+1} = \alpha_2 \\ \frac{1}{2}(\alpha_2^{\ell+1} + \alpha_3^{\ell+1}) = \alpha_3 \end{cases}$$

Solving these equations, we have:

$$\begin{cases} \alpha_0^{\ell+1} = \alpha_0 + \alpha_1 - \alpha_2 - \alpha_3 \\ \alpha_1^{\ell+1} = 2\alpha_2 \\ \alpha_2^{\ell+1} = \alpha_0 - \alpha_1 - \alpha_2 + \alpha_3 \\ \alpha_3^{\ell+1} = -\alpha_0 + \alpha_1 + \alpha_2 + \alpha_3 \end{cases}$$

The matrix that transforms  $\alpha^\ell$  to  $\alpha^{\ell+1}$  is:

$$\alpha^{\ell+1} = \begin{bmatrix} 1 & 1 & -1 & -1 \\ 0 & 0 & 2 & 0 \\ 1 & -1 & -1 & 1 \\ -1 & 1 & 1 & 1 \end{bmatrix} \alpha^\ell.$$

From this configuration, we extract  $C_4$  by analyzing the coefficients of  $\mathbf{v}_0$ ,  $\mathbf{v}_1$ ,  $\mathbf{v}_2$ , and  $\mathbf{v}_3$  in the expanded expression of  $\mathbf{p}$ . Following the same derivation approach, we can similarly determine the remaining coefficient matrices  $C_i$ , as demonstrated below:

$$C_0 = \begin{bmatrix} 1 & -1 & -1 & -1 \\ 0 & 2 & 0 & 0 \\ 0 & 0 & 2 & 0 \\ 0 & 0 & 0 & 2 \end{bmatrix}, \quad C_1 = \begin{bmatrix} -1 & 1 & -1 & -1 \\ 0 & 0 & 2 & 0 \\ 2 & 0 & 0 & 0 \\ 0 & 0 & 0 & 2 \end{bmatrix},$$

$$C_2 = \begin{bmatrix} -1 & -1 & 1 & -1 \\ 2 & 0 & 0 & 0 \\ 0 & 2 & 0 & 0 \\ 0 & 0 & 0 & 2 \end{bmatrix}, \quad C_3 = \begin{bmatrix} -1 & -1 & -1 & 1 \\ 2 & 0 & 0 & 0 \\ 0 & 0 & 2 & 0 \\ 0 & 2 & 0 & 0 \end{bmatrix},$$

$$C_4 = \begin{bmatrix} 1 & 1 & -1 & -1 \\ 0 & 0 & 2 & 0 \\ 1 & -1 & -1 & 1 \\ -1 & 1 & 1 & 1 \end{bmatrix}, \quad C_5 = \begin{bmatrix} 1 & 1 & -1 & -1 \\ 1 & -1 & 1 & 1 \\ 0 & 0 & 0 & 2 \\ -1 & 1 & 1 & -1 \end{bmatrix},$$

$$C_6 = \begin{bmatrix} -1 & -1 & 1 & -1 \\ 1 & 1 & 1 & -1 \\ 0 & 2 & 0 & 0 \\ 1 & -1 & -1 & 1 \end{bmatrix}, \quad C_7 = \begin{bmatrix} -1 & -1 & 1 & 1 \\ 2 & 0 & 0 & 0 \\ -1 & 1 & 1 & -1 \\ 1 & 1 & -1 & 1 \end{bmatrix}.$$

## 2 Sampling for Deformation

Given that our method employs a tetrahedral mesh as a geometric proxy, it naturally inherits the application scenarios of tetrahedra, the most significant of which is the capability to deform objects. In order to render the deformed objects, our approach initially intersects camera rays with the coarse deformed tetrahedral mesh to obtain the sampling points in the deformed space. To ensure the correctness of colors and density, the sampling points and ray directions need to be mapped to the canonical space, where the trained model resides. Thanks to the geometry proxy used for deformation and the tetrahedral mesh used for encoding being the same, there is no need to compute the positions of sampling points in canonical space explicitly. Instead, the barycentric coordinates of the sampling points are calculated in the deformed space. This process is equivalent to transforming a series of sampling points along the ray from the deformed space to the canonical space, as illustrated in Fig. 2.

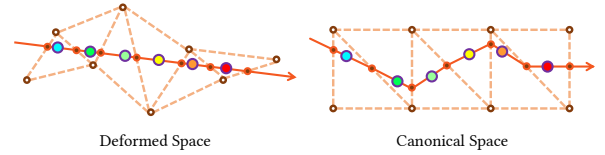

**Figure 2: Mapping Sampling Points from Deformed Space to Canonical Space (2D Illustration).**

## 3 Implementation Details

**Networks Configuration.** Our framework incorporates two MLP networks: the density MLP and the color MLP. The density MLP comprises three hidden layers with 64 neurons each, utilizing Sigmoid activation functions in the hidden layers. The output layer employs an activation mechanism that processes outputs through a truncated exponential function, enhancing stability by regulating extreme values. The color MLP comprises two hidden layers, also with 64 neurons per layer. The hidden layers use ReLU activations to promote non-linearity, while the output employs a Sigmoid function to constrain the RGB values within the  $[0, 1]$  range.

**Metrics Configuration.** We employ Peak Signal-to-Noise Ratio (PSNR) to quantify pixel-level image accuracy. To ensure consistency and comparability of PSNR across normalized image datasets, we explicitly set the range of data to 1. This configuration standardizes the potential maximum value of the signal, thus normalizing all image data within the range from 0 to 1. We also utilize the Structural Similarity Index Measure (SSIM) [8] to evaluate image structural integrity and similarity, which benefits similarly from normalized data inputs. For deeper perceptual analysis, when required, we use Learned Perceptual Image Patch Similarity (LPIPS) [9] with a frozen-parameter VGG network [6] to assess perceptual differences between images. These configurations are uniformly applied across all datasets to ensure consistent evaluation standards and reproducibility of results.

**Loss Function.** We optimize the representation with respect to the mean squared error (MSE) over rendered pixel colors, with

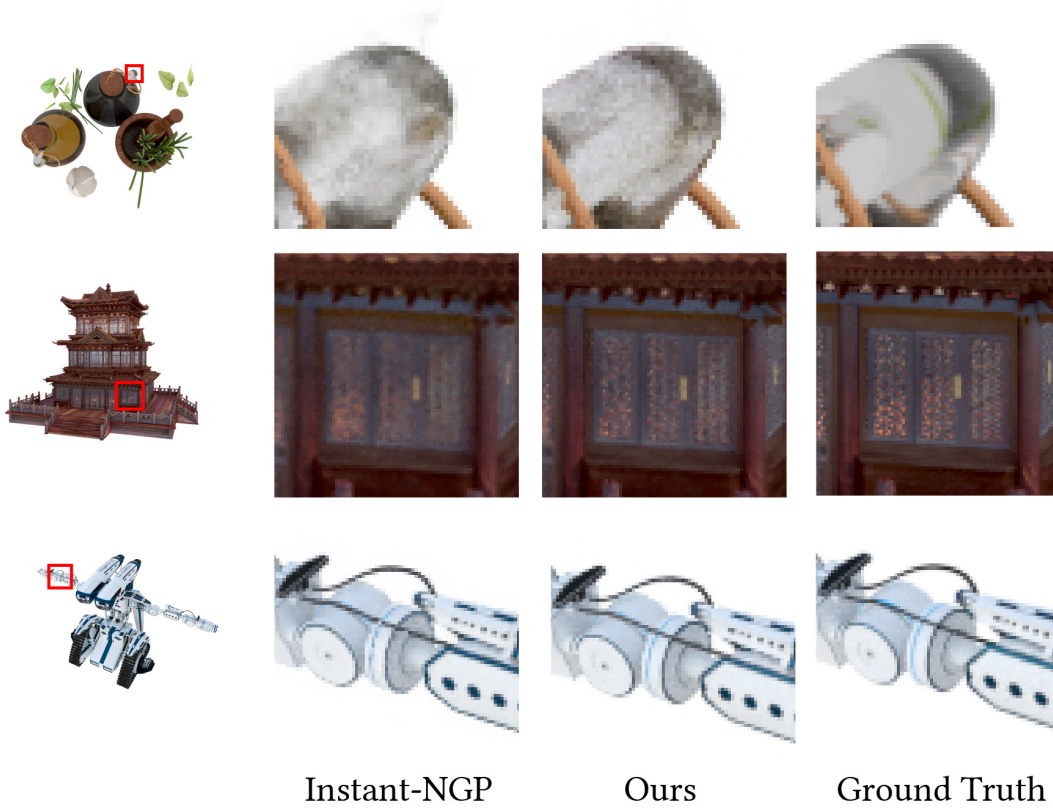

Figure 3: Qualitative Comparisons on the NSVF Dataset [4].

distortion loss proposed by Mip-NeRF 360 [1]. Specifically, the combined loss used to optimize our representation is:

$$\mathcal{L} = \mathcal{L}_{\text{rgb}} + \lambda_{\text{dist}} \mathcal{L}_{\text{dist}}, \quad (3)$$

where the MSE RGB loss  $\mathcal{L}_{\text{rgb}}$  and the distortion loss  $\mathcal{L}_{\text{dist}}$  are:

$$\begin{aligned} \mathcal{L}_{\text{rgb}} &= \frac{1}{|\mathcal{R}|} \sum_{\mathbf{r} \in \mathcal{R}} \|C(\mathbf{r}) - \hat{C}(\mathbf{r})\|_2^2, \\ \mathcal{L}_{\text{dist}}(\mathbf{s}, \mathbf{w}) &= \sum_{i,j} w_i w_j \left| \frac{s_i + s_{i+1}}{2} - \frac{s_j + s_{j+1}}{2} \right| \\ &\quad + \frac{1}{3} \sum_i w_i^2 (s_{i+1} - s_i). \end{aligned} \quad (4)$$

Here  $(s_{i+1} - s_i)$  is the length and  $(s_i + s_{i+1})/2$  is the midpoint of the  $i$ -th query interval. The weight  $w_i$  is for the  $i$ -th sample point. We set the hyperparameter  $\lambda_{\text{dist}}$  to  $1 \times 10^{-2}$  for all scenes.

#### 4 Experiments on NSVF Dataset

In addition to the experimental results presented in the main text, we conduct further experiments on the Synthetic NSVF dataset [4]. We compare these experiments with those from Instant-NGP [5] on metrics such as PSNR, SSIM, and LPIPS. The comparative results are detailed in Table 1.

Fig. 3 illustrates the performance of our method compared to Instant-NGP [5] on the Synthetic NSVF dataset. Visually, our method

Table 1: Quantitative Comparisons on the Synthetic NSVF dataset [4].

|                 | PSNR↑ | SSIM↑ | LPIPS ↓ |
|-----------------|-------|-------|---------|
| Instant-NGP [5] | 35.25 | 0.975 | 0.029   |
| Ours            | 36.51 | 0.979 | 0.024   |

demonstrates superior quality, offering more accurate and detailed reproductions of the scenes.

#### 5 Training Time of Our Method

We compare the training time of DeformRF with the time needed for tetrahedralization [3] after extracting the surface mesh using Instant-NeuS [2]. The training time of DeformRF is shorter. However, Instant-NeuS fails to extract the surface mesh on Tanks and Temples dataset, which is indicated as N/A in the table.

Table 2: Training Time and Tetrahedralizing Time.

|                   | Ours     |          | Tetra-NeRF | Tetrahedralization |
|-------------------|----------|----------|------------|--------------------|
|                   | Stage 1  | Stage 2  |            |                    |
| Synthetic-NeRF    | 1.44 min | 4.21 min | 11.43 hr   | 14.53 min          |
| Tanks and Temples | 1.46 min | 6.16 min | 17.53 hr   | N/A                |

## 6 Memory Usage by Subdivision Levels

Here we provide detailed memory usage concerning different numbers of subdivision levels as shown in Fig. 4.

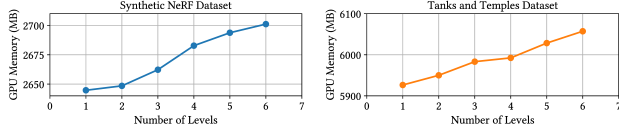

**Figure 4: GPU Memory Usage across Different Numbers of Subdivision Levels.**

## 7 Comparisons with 3D GS

Since the vanilla 3D GS does not support deformation, we conduct an experimental comparison with the derivative work of 3D GS, named GaMeS [7], to show our advantage in the deformation task. Our method demonstrates smoother edges during deformation, whereas 3D GS results in blurred edges. Additionally, 3D GS tends to produce holes when stretched, while ours ensures the continuity and integrity of the object, even under large deformations. These differences arise because our method is based on a continuous neural field, whereas 3D GS is discrete.

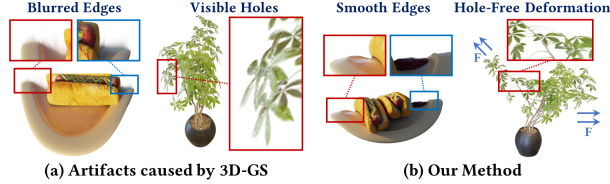

**Figure 5: Comparisons with 3D GS on the Deformation Task.**

## 8 Limitation & Future Work

While our proposed DeformRF method integrates the manipulability of tetrahedral meshes with the high fidelity of feature grid

representations effectively, it is not without its limitations. A primary constraint involves the uniform subdivision of all tetrahedra within the model. Specifically, subdivisions are applied uniformly, regardless of whether the tetrahedra encapsulate critical object details or are positioned within the object’s interior where finer details may not be necessary. This approach results in redundant computational overhead and potentially excessive memory use in areas where high resolution is not required. To address this inefficiency, integrating sparse data structures represents a promising avenue for future research. Sparse data structures can dynamically adjust the level of detail based on the complexity required at different regions within the object. By only subdividing tetrahedra that contribute to visible surface details or are near areas of high geometric complexity, it would be possible to significantly reduce unnecessary computations and memory usage.

## References

- [1] Jonathan T. Barron, Ben Mildenhall, Dor Verbin, Pratul P. Srinivasan, and Peter Hedman. 2022. Mip-NeRF 360: Unbounded Anti-Aliased Neural Radiance Fields. *CVPR* (2022).
- [2] Yuan-Chen Guo. 2022. Instant Neural Surface Reconstruction. <https://github.com/bennyguo/instant-nsr-pl>.
- [3] Yixin Hu, Teso Schneider, Bolun Wang, Denis Zorin, and Daniele Panozzo. 2020. Fast tetrahedral meshing in the wild. *ACM Trans. Graph.* 39, 4, Article 117 (aug 2020), 18 pages. <https://doi.org/10.1145/3386569.3392385>
- [4] Lingjie Liu, Jiatao Gu, Kyaw Zaw Lin, Tat-Seng Chua, and Christian Theobalt. 2020. Neural Sparse Voxel Fields. *NeurIPS* (2020).
- [5] Thomas Müller, Alex Evans, Christoph Schied, and Alexander Keller. 2022. Instant Neural Graphics Primitives with a Multiresolution Hash Encoding. *ACM Trans. Graph.* 41, 4, Article 102 (July 2022), 15 pages. <https://doi.org/10.1145/3528223.3530127>
- [6] Karen Simonyan and Andrew Zisserman. 2015. Very Deep Convolutional Networks for Large-Scale Image Recognition. In *3rd International Conference on Learning Representations, ICLR 2015, San Diego, CA, USA, May 7-9, 2015, Conference Track Proceedings*, Yoshua Bengio and Yann LeCun (Eds.). <http://arxiv.org/abs/1409.1556>
- [7] Joanna Waczyńska, Piotr Borycki, Sławomir Tadeja, Jacek Tabor, and Przemysław Spurek. 2024. GaMeS: Mesh-Based Adapting and Modification of Gaussian Splatting. (2024). [arXiv:2402.01459](https://arxiv.org/abs/2402.01459)
- [8] Zhou Wang, Eero P Simoncelli, and Alan C Bovik. 2003. Multiscale structural similarity for image quality assessment. In *The Thirty-Seventh Asilomar Conference on Signals, Systems & Computers, 2003*, Vol. 2. IEEE, 1398–1402.
- [9] Richard Zhang, Phillip Isola, Alexei A Efros, Eli Shechtman, and Oliver Wang. 2018. The unreasonable effectiveness of deep features as a perceptual metric. In *Proceedings of the IEEE conference on computer vision and pattern recognition*. 586–595.
